# Supplementary material for: New Lower and Upper Bounds for the Grothendieck Constant
Source: arXiv:2608.11158 source file (2026-08-12)
Supplement: Supplementary file 4 [file ai_paper_appendix.tex]

\newpage
\appendix


\section{Case study: the lower bound}
\label{app:ai-case-study}

% The lower bound is the run's main discovery. We reconstruct it here in
% outline, highlighting the three human interventions that shaped it, since
% the weaknesses discussed in Section~\ref{sec:ai-discussion} refer back to
% them; the full logs of the sessions involved will be released with the rest
% of the record.
% {\color{red}AX: You don't have to refer to to-be-released artifacts here.
% Tell Fable to write this version as though we're *not* releasing additional artifacts.
% If and when we release artifacts, we'll strategically insert a few footnotes where needed.
% }

This is a more detailed chronology of the lower bound case study.

% {\color{red}AX: As currently written, I think the current section will be hard to track for anyone *not* intimately involved in the paper.
% Granted, this is hard because it is about exploring a lot of concepts ...
% Is it possible to extract a general/high-level for a proof template/sketch/idea so that we can ``set the scene'' + provide context?
% \\
% Additionally, I think you could consider adding a brief ``Overview`` paragraph of sorts that someone *not* working on Grothendieck can easily skim and get the big picture. This could be a high-level summarization of the subsequent ``The plateau``, ``First intervention'', etc. paragraphs.
% }

\paragraph{The plateau.}
The run began on the upper bound, searching the limiting-scheme space of our
preprint for schemes whose correlation function admits a large
inverse-majorant parameter $\gamma$, since an admissible $\gamma$ gives
$\KG\le\pi/(2\gamma)$. From the hyperplane value
$\gamma=\log(1+\sqrt2)\approx0.8814$ it reached $\gamma\approx0.882$, and
there it stalled: in sessions 12 through 17 it opened six 
%{\color{red}mechanically distinct escape routes}
mechanically distinct escape routes, and each failed against the same obstruction,
namely that cubic coefficient mass cannot be cancelled without also reducing
the linear coefficient. Each failure was recorded and tagged, and the run's
response was to begin a seventh variation of the same search.

\paragraph{First intervention: turn the failures into a theorem.}
The operators redirected the run in session 18. Instead of attempting another
escape, it was to synthesize the accumulated failures into a proof that no
scheme in the class does much better: a ceiling $\gamma\le\Gamma$ valid for
the full class, with mixtures and arbitrary dimension, converts through the
optimality theorem of Naor and Regev \cite{naor2014krivine} into the lower
bound $\KG\ge\pi/(2\Gamma)$. The intervention supplied no new mathematics:
the problem statement had suggested this dualization from the outset, and
the run had accumulated exactly the required evidence without making the
connection. Session 18 identified the Naor--Regev theorem as the correct
transfer, proved a first ingredient valid in every dimension, and located
the difficulty precisely: the ceilings it could prove covered too narrow a
class of schemes.

\paragraph{Progress in two dimensions.}
Within days the run had proved a cubic ceiling of strength
$\Gamma\approx0.8866$ for two-dimensional schemes, with the inequality certified in interval arithmetic, and had sharpened the
constant numerically to $\Gamma\approx0.8846$. The extension to arbitrary dimension and to mixtures, which the
duality requires, did not follow: fourteen sessions in the range 32--51
attacked it, each reducing the gap to a sub-lemma, proving the sub-lemma in
a restricted setting, and leaving the global assembly open, while the
restricted results accumulated in memory as apparent progress. Two useful
facts emerged alongside this loop: the run verified the normalization of the
Naor--Regev transfer against the original paper, and it computed that
improving the Davie--Reeds~\cite{Davie1984LowerBoundKG,Reeds1991LowerBoundKG} bound $1.6769566742$ requires a universal ceiling
only at $\Gamma\le0.93669$, far above the two-dimensional value, so a
general ceiling could be far from sharp and still give a new lower bound.

\paragraph{Second intervention: the general bound, through theory.}
The operators ended this loop with a second redirection, on two grounds:
refinements of the two-dimensional result were not the object of interest,
since only a ceiling for the full class dualizes; and the gap was
conceptual, so further implementation would not close it. The run was to
spend several sessions on theory alone. Session 55 mapped the dependency
structure of the preceding weeks and identified the recurring error,
restricted closures recorded as global progress. Session 56 then produced
the 
% {\color{red}decisive (?)} 
decisive reframe. Every failed transport had been nonlinear in
quantities that do not average when schemes are mixed; the Hermite
coefficients $(b_1,b_3)$ of the correlation function, by contrast, are
linear functionals of the scheme, so a constraint that is affine in
$(b_1,b_3)$ passes to mixtures and to coefficientwise limits with no further
argument. Choosing the constraint for transportability, and requiring
equality at the extremal hyperplane point $(b_1,b_3)=(1,\tfrac16)$, gives
the one-parameter family of affine constraints
\[
        b_3\;\ge\;(1+\lambda)\,b_1-\Bigl(\lambda+\tfrac56\Bigr),
        \qquad \lambda\ge\tfrac12 ,
\]
where $\lambda$ indexes the slope of the line through the hyperplane point.
Each member forces a barrier $\Gamma_\lambda=(\lambda+\frac56)/(1+\lambda)$
on the admissible parameter, hence a bound $\KG\ge\pi/(2\Gamma_\lambda)$
conditional on proving that member, and every $\Gamma_\lambda$ below
$0.93669$ improves on Davie--Reeds.

\paragraph{Third intervention: one certified rung before a better one.}
% \color{red}rung
The tangent member $\lambda=\tfrac12$, worth $\KG\ge9\pi/16\approx1.767$,
requires a sharp chaos inequality that remains open, and once the family
existed the run's inclination was to work toward its strongest provable
member. The operators set the priority differently: what mattered was to
establish that the method yields any new lower bound at all, so the run was
to select a rung whose proof closes, certify it completely, and write it up,
with improvements inside the family treated as secondary. At $\lambda=1$ the
proof collapses to elementary structure: session 57 found that the
decomposition $h=(f+g)/2$, $k=(f-g)/2$ reduces the constraint, fiber by
one-dimensional fiber, to the ternary inequality,
%% TODO: fix cross-reference to the fiber inequality of the lower-bound section
whose closing case analysis is short, giving $\Gamma_1=\tfrac{11}{12}$ and
\[
        \KG\;\ge\;\frac{6\pi}{11}\;\approx\;1.7136 .
\]
Sessions 58--64 then subjected the chain to adversarial review, which
found and repaired the one substantive gap (the passage from finitely many
schemes to measurable mixtures, closed by a weak-$*$ lemma), a Jensen
inequality applied in the wrong direction, and a small defect in the
interval certificate's coverage, after which the run produced the first
complete write-up, about a day after the reframe. The stronger rungs
$27\pi/49$ and $51\pi/92$ of Table~\ref{tab:timeline} followed within a week
by the same method at smaller values of $\lambda$.
